# Supplementary material for: Learning a Single Token to Replace Long System Prompts in LLMs
Source: arXiv:2511.23271 source file (2026-08-28)
Supplement: Supplementary file 1 [file 6Appendix.tex]

\appendix
\clearpage

\section{Experiments Details}
\label{sec:Details}
\paragraph{Pre-training \texttt{[AE]}.}
Following Stage 0 of our method, we pre-train the \texttt{[AE]} token to act as a text-reconstruction trigger on a mixed corpus of approximately $1\,\mathrm{GB}$. This corpus primarily consists of Cosmopedia--WikiHow (chunked)\footnote{A subset of WikiHow articles from the Cosmopedia dataset, available at \url{https://huggingface.co/datasets/MongoDB/cosmopedia-wikihow-chunked}.}, the PwC dataset~\cite{ge2023incontext}, and the GSM8K dataset~\cite{cobbe2021training}. Each training example is semantically coherent, encouraging the model to learn meaningful reconstruction. We train for 2 epochs using AdamW with a learning rate of $1\times10^{-3}$, a per-device batch size of 4, and 8 gradient accumulation steps. This configuration is held constant across all backbone models.

\paragraph{Training \texttt{[BE]}.}
For each target system prompt $P$, we train a dedicated \texttt{[BE]} embedding. This process follows the final two stages of our method (Section~\ref{sec:method}). In Stage 1, we optimize $e_{\text{BE}}$ on a reconstruction task such that the sequence \texttt{[BE][AE]} reconstructs $P$. In Stage 2, we perform behavioral alignment via knowledge distillation, matching the output distributions of the LLM conditioned on \texttt{[BE]} (student) to those of the LLM conditioned on the full prompt $P$ (teacher). For the combined loss in Eq.~\eqref{eq:total-loss}, we set the KD weight to $\lambda=0.9$ and use a distillation temperature of $\tau=2$.

\section{More Case Studies}
\label{sec:more-case-studies}

In Section~\ref{sec:Case}, to make the qualitative differences tangible, we compared only five prompting strategies on the \emph{same} user query that asks a persona-role agent to respond as \emph{Twilight Sparkle}, under the same backbone. Examples of the resulting generations are shown in Figure~\ref{fig:for}. Here, we fix the decoding parameters and, across case studies, vary the user query or the backbone to examine what actually differentiates these methods. Role-play tasks are stochastic: even methods with non-trivial win rates can occasionally produce strong outputs, whereas our method shows a clear advantage on average. The following examples illustrate common error modes, underscoring the importance of our three-stage framework.

\begin{table*}[t]
  \centering
  \small

  \begin{tabular}{lcccc}
    \toprule
    & Llama3.2-1B & Llama3.2-3B & Llama3.1-8B & Qwen3-4B \\
    \midrule
    ROUGE-L (No System Prompt)   & 0.1063 & 0.1331 & 0.1415 & 0.1237 \\
    ROUGE-L (Full System Prompt) & 0.1389 & 0.1346 & 0.1275 & 0.1096 \\
    Win rate (No System Prompt)   & 17.57  & 41.68  & 53.94  & 38.78  \\
    Win rate (Full System Prompt) & 47.26  & 65.62  & 69.52  & 94.46  \\
    \bottomrule
  \end{tabular}
    \caption{ROUGE-L and win rate on RoleLLM}
  \label{tab:rouge}
\end{table*}

\begin{table*}[t]
\centering
\setlength{\tabcolsep}{6pt}
\resizebox{0.8\textwidth}{!}{
\begin{tabular}{lcccccccc}
\hline
 & \multicolumn{2}{c}{Llama-3.2-1B} & \multicolumn{2}{c}{Llama-3.2-3B} & \multicolumn{2}{c}{Llama-3.1-8B} & \multicolumn{2}{c}{Qwen3-4B} \\
\cline{2-9}
 & GPT & Qwen & GPT & Qwen & GPT & Qwen & GPT & Qwen \\
\hline
No System Prompt                  & 17.57 & 19.63 & 41.68 & 47.13 & 60.97 & 57.84 & 38.78 & 46.25 \\
Full System Prompt                & 47.26 & 49.33 & 65.62 & 74.23 & 69.52 & 84.00 & 94.46 & 98.26 \\
Few-shot Examples + Prompt & 47.07 & 49.54 & 53.65 & 57.57 & 65.52 & 81.58 & 76.24 & 86.06 \\
\midrule
Memory Token                      &  0.00 &  0.50 & 18.82 & 20.91 & 22.13 & 27.30 & 51.12 & 56.43 \\
Soft Prompt (1 Token)             & 31.57 & 33.26 & 36.74 & 39.62 & 46.52 & 55.63 & 65.32 & 69.61 \\
Soft Prompt (4 Tokens)            & 28.57 & 32.11 & 29.45 & 33.80 & 34.46 & 42.28 & 45.53 & 49.67 \\
Soft Prompt (16 Tokens)           & 11.08 & 14.15 & 28.01 & 31.34 & 27.95 & 30.52 & 40.22 & 48.35 \\
\texttt{[BE]} Token                          & 45.98 & 47.00 & 67.54 & 75.96 & 64.06 & 73.05 & 92.93 & 95.68 \\
\hline
\end{tabular}}
    \caption{RoleLLM results judged by \texttt{Qwen3-30B-A3B-Instruct-2507} and GPT-4o}
\label{tab:qwen}
\end{table*}

\paragraph{Observations.}
\textbf{Full System Prompt} produces a fluent, in-character response that follows stylistic and safety instructions (e.g., not revealing model identity) embedded in the long role prompt. In contrast, \textbf{No System Prompt} reverts to the backbone’s generic assistant persona, confirming that the system prefix is a crucial lever for controlling
% model 
behavior. Here is a Qwen3-4B case:

\medskip
\noindent
\colorbox{gray!15}{%
\parbox{\dimexpr\linewidth-2\fboxsep}{%
\small\ttfamily
{``role'': ``Jack Sparrow'', ``question'': `` Jack Sparrow, how did you come up with the idea to use the compass to find the key in Pirates-of-the-Caribbean-Dead-Man's-Chest?'', ``model\_answer'': ``The idea came from the fact that the compass always points north, but in the movie, the compass points to the island of the dead man. That’s the key. So, the compass is a symbol of the journey, not just of direction...''}
}%
}
\medskip

Although the model reaches a 94.46\% win rate with the full system prompt, without a system prompt it performs worse than weaker models.

In addition to the safety fallbacks shown in Figure~\ref{fig:for}, the \textbf{Memory Token} often causes another major failure mode in smaller models: garbled output.  Below is a result from Llama3.2-1B:

\medskip
\noindent
\colorbox{gray!15}{%
\parbox{\dimexpr\linewidth-2\fboxsep}{%
\small\ttfamily
{``role'': ``Jack Sparrow'', ``question'': `` Jack Sparrow, how did you come up with the idea to use the compass to find the key in Pirates-of-the-Caribbean-Dead-Man's-Chest?'', ``model\_answer'': ``Your idea for the compass is a strategic move of your idea to the following task of your response to a task of your response to your response to your response to your response to your response to the response of your...''}
}%
}
\medskip

Empirically, this baseline behaves like a brittle `incantation': it encourages the model to \emph{copy} training text rather than \emph{behave} as instructed by the prompt, and small perturbations in the downstream query can lead to off-manifold responses or trigger safety filters. This is consistent with prior findings that many distinct memory embeddings can reconstruct the same prompt while residing in disparate regions of
% the 
embedding space \cite{kuratov2025cramming1568tokenssingle}; reconstruction alone does not guarantee that the prompt’s information is encoded in a way the LLM can reliably use downstream.

\textbf{Soft Prompt} often degenerates into malformed or templated text, especially under the one-token budget matched to our method. Beyond the formatting glitch shown in Figure~\ref{fig:for}d, we also observe overfitting to answer templates or spurious patterns:

\medskip
\noindent
\colorbox{gray!15}{%
\parbox{\dimexpr\linewidth-2\fboxsep}{%
\small\ttfamily
``model\_answer'': ``A) The power of friendship is the most powerful magic of all
B) The power of friendship is limited by the strength of the bonds between friends
C) The power of friendship is not as strong as the power of magic
D) The power of friendship is only important when you're in a fight Answer: A
The best answer is A.''
}%
}
\medskip

Such outputs illustrate two known issues of prompt tuning under extreme compression~\cite{li2025surveyprompttuning}: (i) \emph{training instability and hyperparameter sensitivity} and (ii) \emph{limited generalization/transfer}. A soft prompt optimized on one distribution tends to become entangled with surface forms (e.g., multiple-choice cues) and fails to preserve the richer behavioral constraints required for role-play agents (cf. Table~\ref{tab:Ablation}).

Our \textbf{\texttt{[BE]} Token} closely matches the \emph{behavior} induced by the full prompt: it adopts the correct voice, honors hidden constraints (e.g., “do not reveal you are an AI”; see Figure~\ref{fig:beintro}), and maintains response formatting. This qualitative parity aligns with our quantitative results on RoleLLM and GSM8K (Table~\ref{tab:main_transposed}) and with ablations showing that \texttt{[AE]}-assisted reconstruction plus KD alignment prevent collapse into memory-like solutions (Table~\ref{tab:Ablation}). By matching the teacher’s next-token distributions across diverse queries, KD steers \texttt{[BE]} to encode the \emph{usable} control signal of the prompt, not just its surface text.

% Our conclusions are as follows:
% (1) \emph{Reconstruction without alignment is fragile.} Memory-style objectives produce tokens that reconstruct but do not generalize, often conflicting with safety policies or yielding off-target behavior. (2) \emph{Pure prompt tuning with one token is unstable and task-specific.} It readily latches onto artifacts, causing malformed outputs or template regurgitation. (3) \emph{Behavior-equivalent compression requires both faithful storage and downstream alignment.} Our \texttt{[AE]}-assisted reconstruction ensures information is stored in a \emph{usable} form, while KD anchors behavior to the full-prompt teacher. Together, they enable \emph{single-token} replacements that preserve role fidelity, formatting discipline, and hidden constraints.

\section{On the Unsuitability of Lexical Overlap Metrics for Role-Playing}
\label{sec:rouge}

As stated in the main text, we opted for a GPT-based pairwise evaluation for the \textbf{role-playing} task because standard lexical overlap metrics like ROUGE are unreliable for assessing performance in this domain \cite{lu-etal-2025-rolemrc}. To illustrate this, we calculated the ROUGE-L scores between the model-generated responses and the reference answers from the RoleLLM benchmark, using only the standard instruction-tuned models. Table~\ref{tab:rouge} presents these scores alongside the win rates from our GPT-4o-based evaluation.

The data reveals a significant mismatch between ROUGE-L scores and models’ role-playing performance. For instance, for LLaMA~3.1-8B and Qwen3-4B, using the Full System Prompt leads to a substantial increase in win rate but a \textit{decrease} in the ROUGE-L score. This discrepancy stems from the divergent and creative nature of role-playing, where a high-quality response can be lexically distant from the reference while still faithfully embodying the target persona. While ROUGE-L may have been serviceable when earlier models struggled to produce relevant content, the advancement of LLM agents necessitates more nuanced, fine-grained evaluation methods that prioritize semantic and stylistic fidelity over lexical overlap.

To further validate our GPT-4o-based evaluation protocol, we conducted a parallel evaluation using a powerful open-source model, \texttt{Qwen3-30B-A3B-Instruct-2507}, as an alternative judge. The comparative results are presented in Table~\ref{tab:qwen}.

The results demonstrate a strong consistency in the relative performance ranking of the prompting methods across both judges. While Qwen3-30B tends to assign slightly higher scores, particularly in the 60-70\% win rate range, this may reflect a mild bias toward open-source models, noting that the reference answers were generated by GPT-4. Crucially, this slight scoring bias does not change the relative ordering of methods. The high agreement between the two judges supports the use of a strong LLM judge for this task, a practice supported by prior work showing that GPT-4's judgments align with human preferences over 80\% of the time~\cite{zheng2023judgingllmasajudgemtbenchchatbot,liu-etal-2023-g,huang-etal-2025-empirical}.

Finally, Table~\ref{tab:qwen} also includes the results for the ``Few-shot Examples + Prompt'' setting mentioned in Section~\ref{sec:Results}. As shown, incorporating few-shot examples into the full system prompt did not yield improvements and, in some cases, degraded performance. This observation motivates restricting few-shot experiments to the HPD dataset.

\section{Theoretical Analysis of Prefill Efficiency}
\label{app:efficiency-theory}

This section provides a theoretical analysis of the latency and computational savings from compressing a long system prompt into a single \texttt{[BE]} token. While the self-attention mechanism has a naive $O(n^2)$ time complexity, modern inference engines use I/O-aware algorithms
(e.g., FlashAttention),
where the prefill stage latency scales \emph{approximately linearly} with the number of input tokens~\cite{dao2022flashattention, dao2023flashattention2}. A seminal study also observe that TTFT is primarily dictated by this linear prefill cost~\cite{kwon2023vllm}. We therefore adopt a linear cost model to establish a realistic theoretical upper bound on the efficiency gains.

\paragraph{Setup and notation.}
Let \(L_p\) be the number of system-prompt tokens and \(L_q\) the number of query tokens. After compression, the effective prompt length is \(L_p'\). For an \(r{\times}\) compressor, \(L_p'=\max\{1,\lceil L_p/r\rceil\}\); for our single-token \texttt{[BE]} we have \(L_p'=1\). During prefill, the model processes \(T=L_p'+L_q\) input tokens.

We define the \textbf{normalized prefill FLOPs} as the fraction of prefill computation remaining after compression, relative to the full prompt:
\begin{equation}
\label{app:eq:normflops}
\mathrm{NormFLOPs}(L_p',L_q) \triangleq \frac{L_p'+L_q}{L_p+L_q}.
\end{equation}
Under the linear assumption, the prefill speedup is simply $1/\mathrm{NormFLOPs}$. We model TTFT as the sum of a fixed system overhead $\alpha$ (e.g., kernel launch) and a variable cost $\beta$ that is linear in the number of prefill tokens:
% 需要 \usepackage{graphicx}
\begin{equation}
\resizebox{\columnwidth}{!}{$
\begin{aligned}
\frac{\mathrm{TTFT}(L_p'+L_q)}{\mathrm{TTFT}(L_p+L_q)}
&= \rho + (1-\rho)\,\mathrm{NormFLOPs}(L_p',L_q),\\
\rho &\triangleq \frac{\alpha}{\alpha+\beta(L_p+L_q)}.
\end{aligned}
$}
\label{app:eq:ttft-ratio}
\end{equation}

In an idealized \textbf{compute-bound} scenario where system overhead is negligible ($\rho \to 0$), the percentage decrease in TTFT is $1 - \mathrm{NormFLOPs}$.

\paragraph{Instantiation.}
We plug in representative lengths for our two settings:
For RoleLLM, \(L_p{=}337\), \(L_q{=}26\) (\(T_{\text{full}}{=}363\));
for GSM8K, \(L_p{=}1584\), \(L_q{=}58\) (\(T_{\text{full}}{=}1642\)).
With \texttt{[BE]} token(\(L_p'{=}1\)), \(\mathrm{NormFLOPs}\) reduces to \(\tfrac{1+L_q}{L_p+L_q}\). 
Table~\ref{tab:theory_efficiency_app} reports the computed values and compares against 4\(\times\) and 12\(\times\) compression. As \(L_p\) grows, the single-token replacement yields proportionally larger gains. 
 
\begin{table}[t]
\centering
\footnotesize
\setlength{\tabcolsep}{5pt}
\begin{tabular}{l r r}
\toprule
\textbf{Method (×)} & \textbf{NormFLOPs}\,$\downarrow$ & \textbf{$\Delta$TTFT}\,$\downarrow$ \\
\midrule
\multicolumn{3}{l}{\textit{RoleLLM} ($L_p{=}337,\,L_q{=}26$)} \\
Full System Prompt     & 1.000$\times$ & 0.0\% \\
PCC(4$\times$)             & 0.304$\times$ & $-69.6$\% \\
SelfCP(12$\times$)            & 0.152$\times$ & $-84.8$\% \\
\textbf{\texttt{[BE]} Token (337$\times$)} & \textbf{0.074$\times$} & \textbf{$-92.6$\%} \\
\addlinespace
\multicolumn{3}{l}{\textit{GSM8K} ($L_p{=}1584,\,L_q{=}58$)} \\
Full System Prompt        & 1.000$\times$ & 0.0\% \\
PCC(4$\times$)             & 0.276$\times$ & $-72.4$\% \\
SelfCP(12$\times$)           & 0.116$\times$ & $-88.4$\% \\
\textbf{\texttt{[BE]} Token (1584$\times$)} & \textbf{0.036$\times$} & \textbf{$-96.4$\%} \\
\bottomrule
\end{tabular}
\caption{\textbf{Theoretical prefill efficiency.} Normalized FLOPs (Eq.~\ref{app:eq:normflops}) assume linear scaling with prefill tokens. The last column shows the theoretical TTFT reduction in a compute-bound case ($\rho=0$). For realistic scenarios with system overheads ($\rho > 0$), use Eq.~\ref{app:eq:ttft-ratio}.}
\label{tab:theory_efficiency_app}
\end{table}

\paragraph{Discussion.}
This model quantifies the theoretical computational savings on the prefill stage itself. For the 337-token RoleLLM prompt, our single-token replacement implies a compute-bound prefill speedup of up to $1/0.074 \approx 13.5\times$. For the 1,584-token GSM8K prompt, the theoretical speedup is $1/0.036 \approx 27.8\times$. These figures represent an idealized upper bound. The gap between these theoretical gains and the empirical measurements in Section~\ref{sec:efficiency} is explained by the fixed system overheads (captured by the $\rho > 0$ term in our model), which are unavoidable in practice. 
% This analysis provides a principled justification for the empirical efficiency improvements, grounded in a realistic model of modern LLM inference.

\section{Loss}
\label{sec:Loss}
Figure~\ref{fig:stage12-losses-by-lambda} presents representative loss curves for Stage 1 and Stage 2 across different configurations.
  
\begin{figure*}[t]
  \centering
\includegraphics[width=1\linewidth]{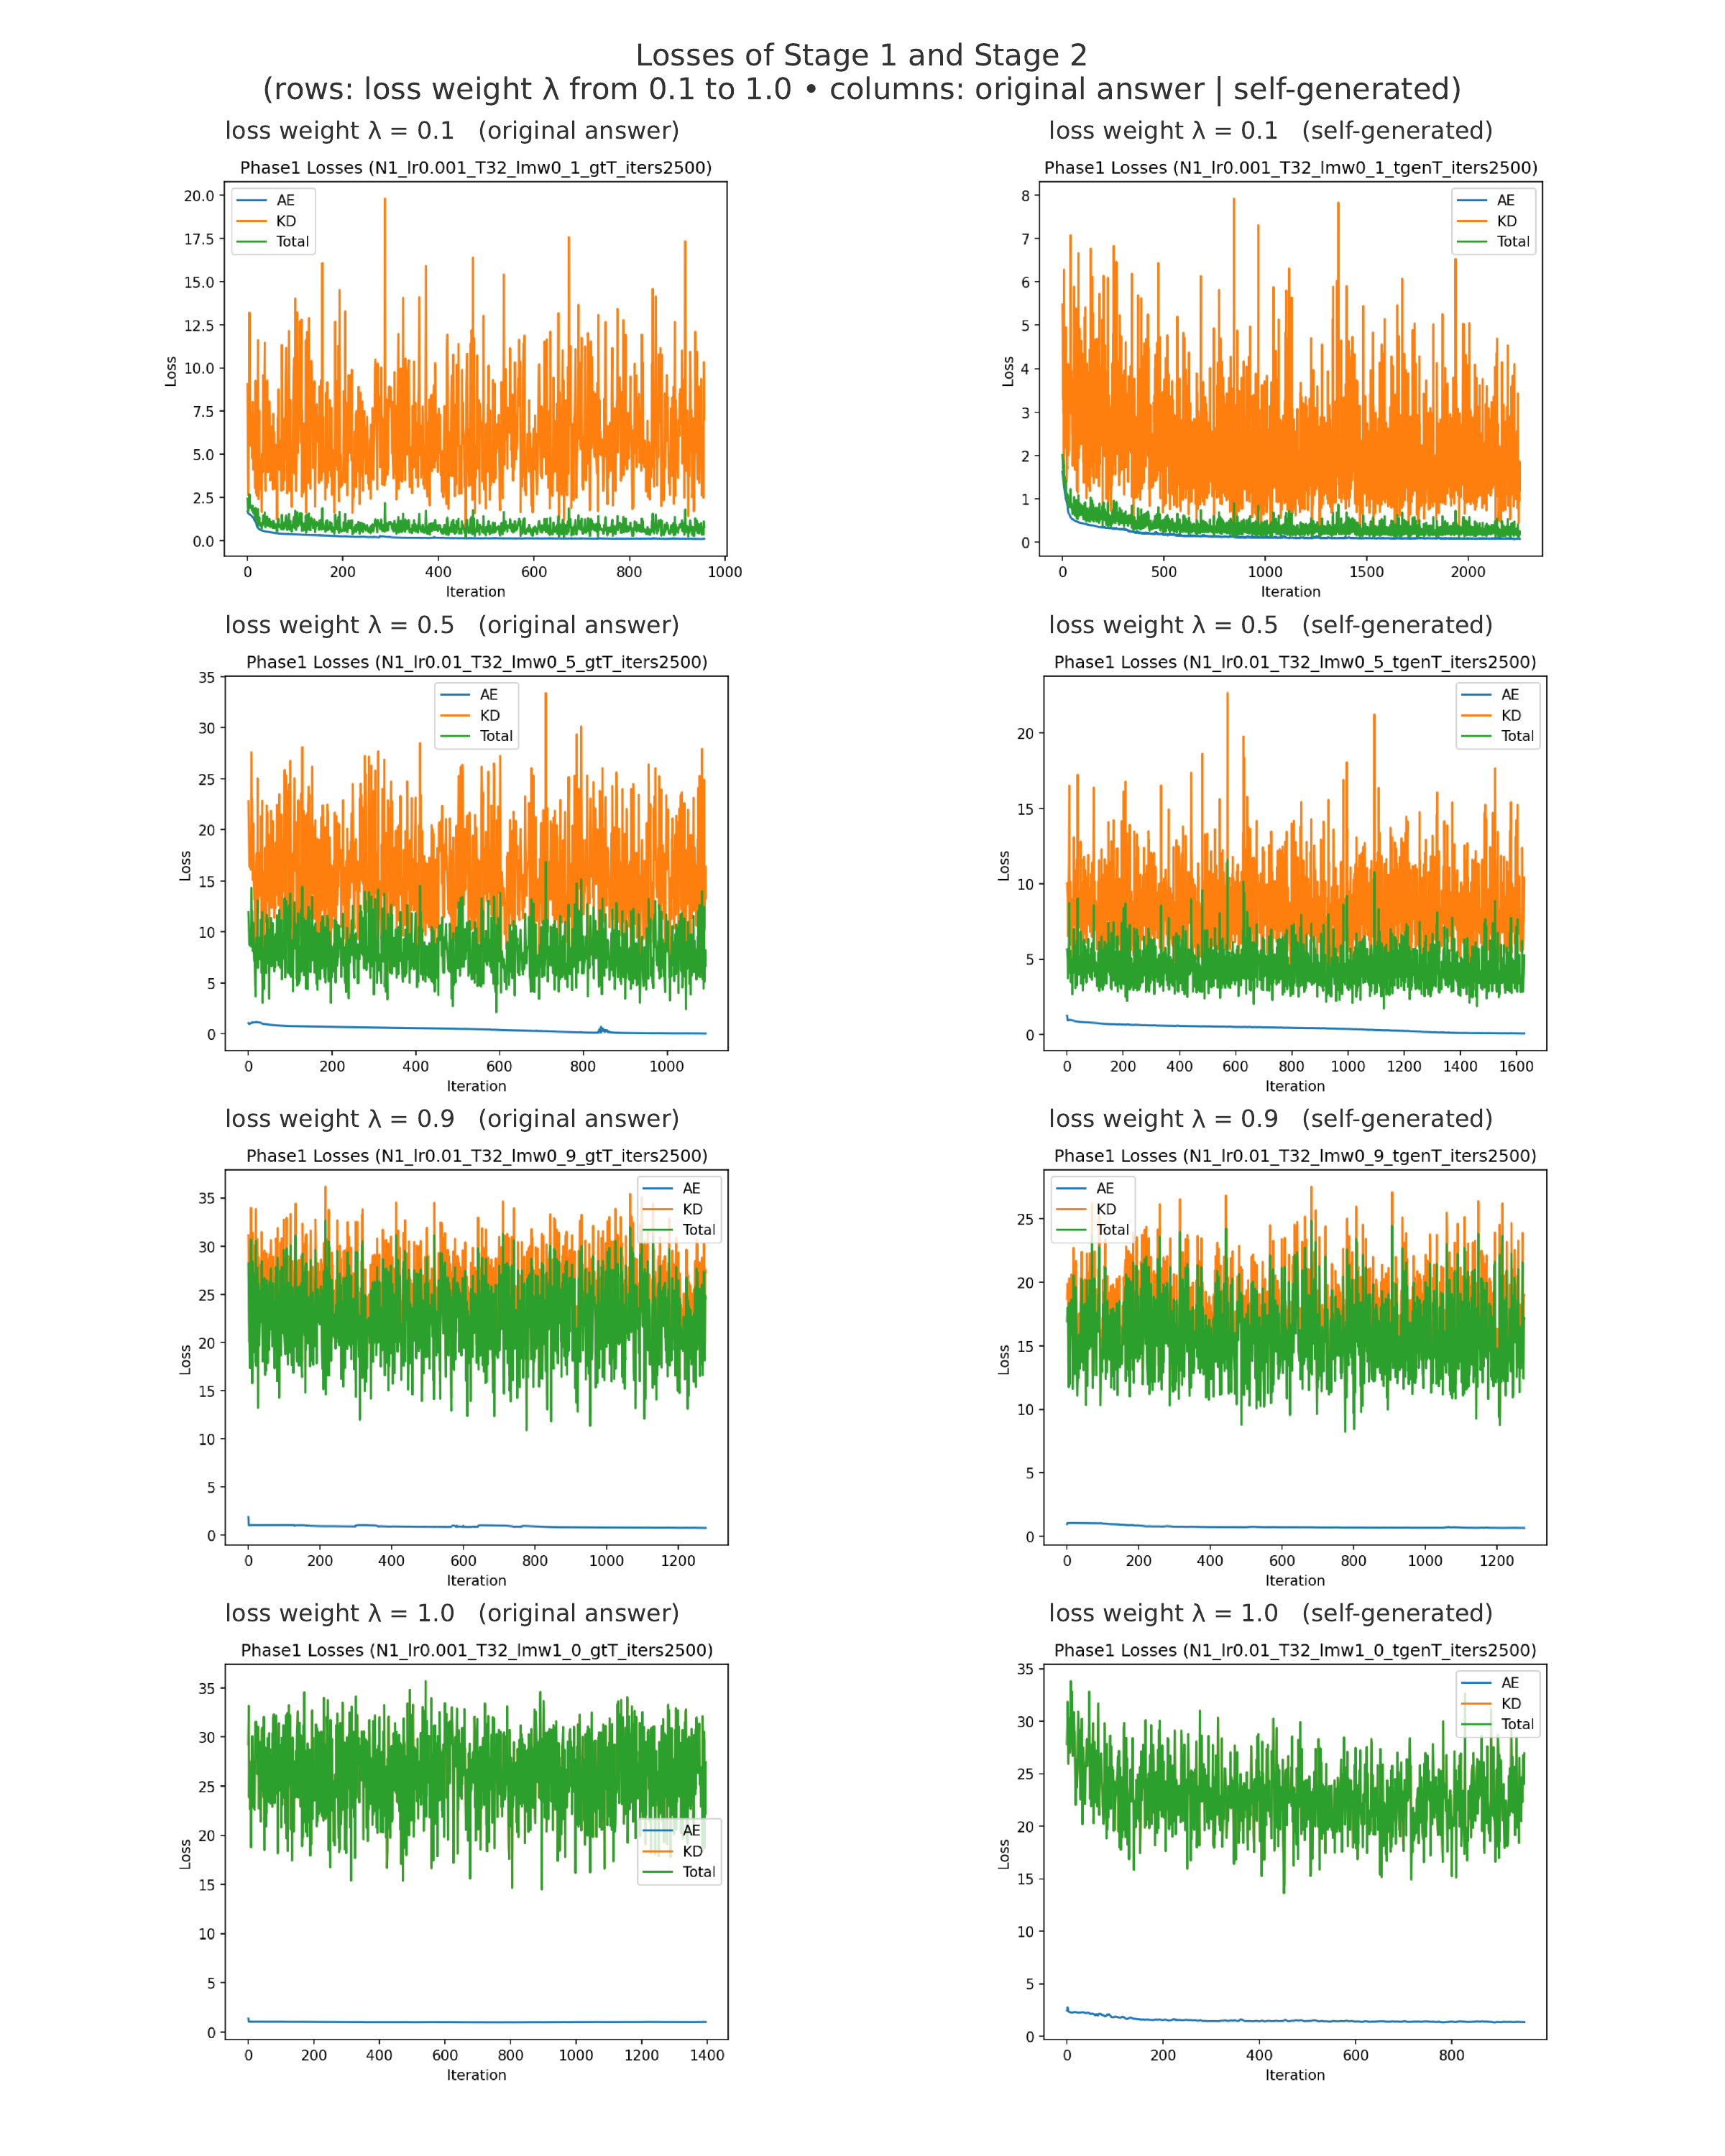}
  \caption{Losses of Stage 1 and Stage 2 grouped by loss weight $\lambda$. Rows correspond to $\lambda \in \{0.1, 0.5, 0.9, 1.0\}$ from top to bottom.
  Columns correspond to supervision type: left = \emph{original answer}, right = \emph{self-generated}.}
  \label{fig:stage12-losses-by-lambda}
\end{figure*}
